# Supplementary material for: Pedagogical Alignment of Large Language Models
Source: arXiv:2402.05000 source file (2024-10-05)
Supplement: Supplementary file 1 [file appendix.tex]

% \subsection{Data analysis}
% In this section, we provide comprehensive statistics on the data distribution of the dataset across three classification fields - Evaluation of Student Response, Action based on Evaluation, and Subproblem State.

% \begin{figure}[h!]
%     \centering
%     % First subfigure with eval_chart.pdf
%     \begin{subfigure}[b]{0.48\textwidth}
%         \centering
%         \includegraphics[width=\textwidth]{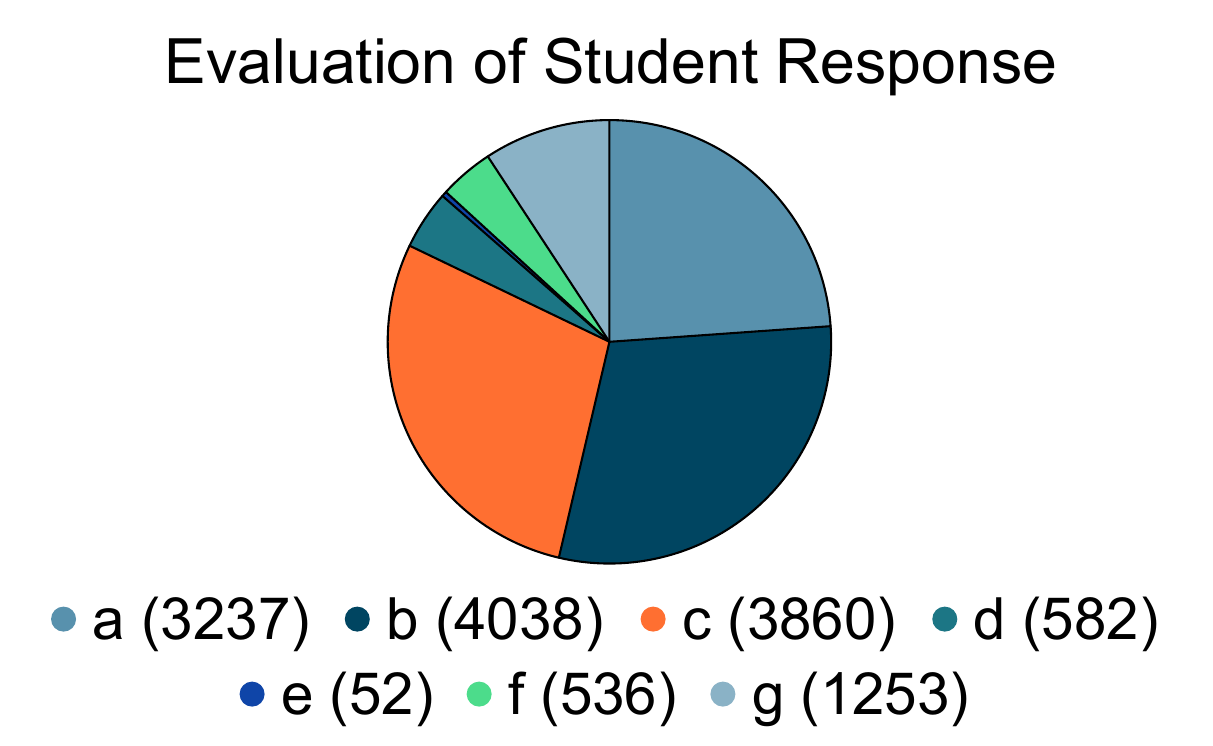}
%         \label{fig:evalChart}
%     \end{subfigure}
%     \hfill % Adds horizontal space between the two subfigures
%     % Second subfigure with action_chart.pdf
%     \begin{subfigure}[b]{0.48\textwidth}
%         \centering
%         \includegraphics[width=\textwidth]{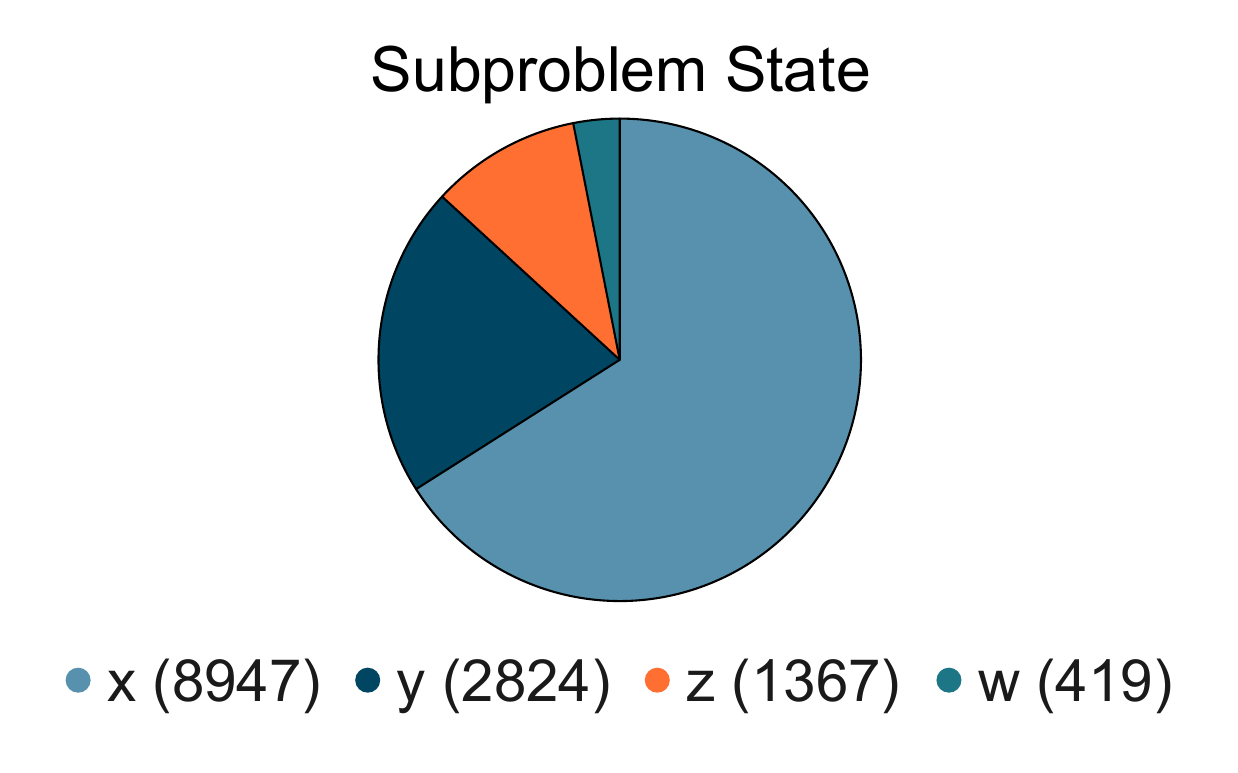}
%         \label{fig:actionChart}
%     \end{subfigure}
%     \\
%     % Third subfigure with subproblem_chart.pdf, vertically below the first two
%     \begin{subfigure}[b]{\textwidth} % Takes the full text width
%         \centering
%         \includegraphics[width=0.7\textwidth]{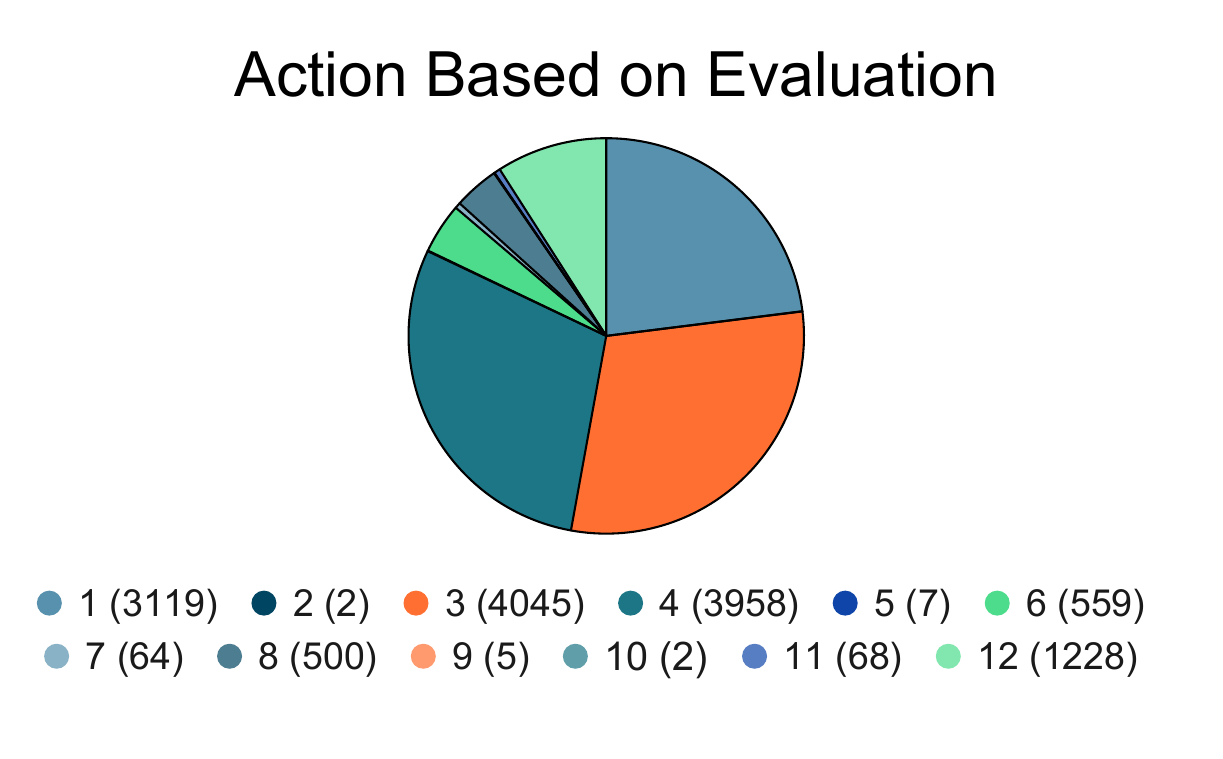} % Adjust width as needed
%         \label{fig:subproblemChart}
%     \end{subfigure}
    
%     \caption{Overview of the data distribution of three classification fields - Evaluation of Student Response, Action based on the Evaluation, and Subproblem State.}
%     \label{fig:charts}
% \end{figure}

\subsection{SFT vs DPO, IPO, and KTO}

\begin{table}[h!]
\vspace{2mm}
\label{tab:app_exp1}
\centering
\resizebox{0.95\columnwidth}{!}{
\begin{tabular}{|l|c|c|c|c|}
\hline
\textbf{Model}               & \textbf{SFT} & \textbf{DPO} & \textbf{IPO} & \textbf{KTO}  \\ \hline
Mistral & 0.34 (0.42,0.24,0.37)     & \textbf{0.56} (0.63,0.37,\textbf{0.67})     & 0.48 (0.56,0.33,0.56)     & 0.55 (0.62,0.37,0.65)     \\
Vicuna      & 0.54 (0.64,0.37,0.60)     & 0.55 (\textbf{0.65},\textbf{0.39},0.62)    & 0.55 (0.65,\textbf{0.39},0.62)     & 0.54 (0.64,0.37,0.61)     \\
Zephyr       & 0.14 (0.21,0.12,0.10)      &\textbf{0.56} (\textbf{0.65},0.38,0.66)     & 0.26 (0.32,0.19,0.28)     & 0.54 (0.63,0.37,0.63)   \\ \hline
\end{tabular}
}
\caption{SFT vs DPO, IPO, KTO. Each cell shows the average f1-score across three classification fields - Evaluation of student response, Action based on the evaluation, and Subproblem State, respectively.
We observed that for Mistral (Mistral-7B-Instruct-v0.2) and Zephyr (zephyr-7b-beta), all three RL alignment algorithms - DPO, KTO, and IPO - showed notable gains in f1-score across all fields as compared to SFT.
Across both models, DPO and KTO outperformed IPO. For Vicuna (vicuna-7b-v1.5), all three algorithms performed roughly the same.
% These results highlighted the significant impact of alignment algorithms, particularly DPO and KTO, in boosting the accuracy of state-of-the-art models.
}
\end{table}

To further support the observations in Section \ref{exp1}, we measured the f1-scores of three classification fields in the responses: Evaluation of Student Response, Action based on Evaluation, and Subproblem State.

We observed significant accuracy improvements on Mistral and Zephyr SFT models. Specifically, Mistral demonstrated improvements of 0.22, 0.14, and 0.21 from DPO, IPO, and KTO respectively, while Zephyr showed improvements of 0.42, 0.12, and 0.40 respectively (Table  \ref{tab:app_exp1}). Notably, for both Mistral and Zephyr, DPO and KTO significantly outperformed IPO. However, the Vicuna model, already noted for its high SFT performance, showed only marginal improvements from the alignment; all three algorithms exhibited roughly similar performance.
Our results are in alignment with the findings of similar studies \citep{preftuningblog}, which have reported superior performance of DPO and KTO over IPO on Zephyr when the model was fine-tuned on preference datasets, such as Intel’s ORCA dataset pairs \citep{OpenOrca} and the Ultra-Feedback dataset \citep{tunstall2023zephyr}.

This experiment underscored the pivotal role of alignment algorithms in improving the accuracy of SFT models. Mistral and Zephyr, the top performing models, exhibited pronounced improvements over Vicuna. Therefore, we demonstrated the efficacy of pedagogical alignment on state of the art models.

\subsection{Effect of beta on DPO and IPO}

\begin{figure}[h!]
    \centering
    \begin{subfigure}[b]{0.49\textwidth}
        \centering
        \includegraphics[width=\textwidth]{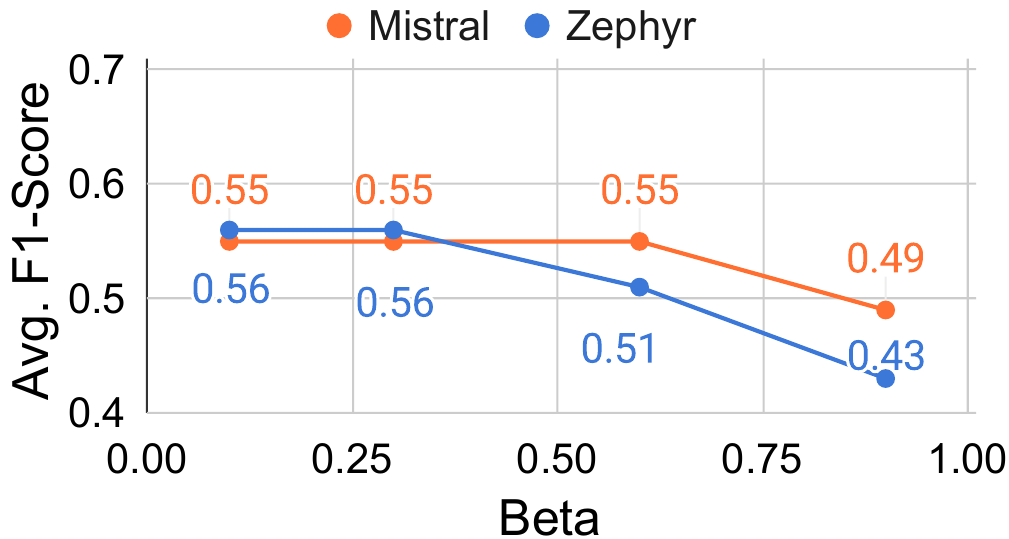}
    \end{subfigure}
    \hfill % or \quad for some space
    \begin{subfigure}[b]{0.49\textwidth}
        \centering
        \includegraphics[width=\textwidth]{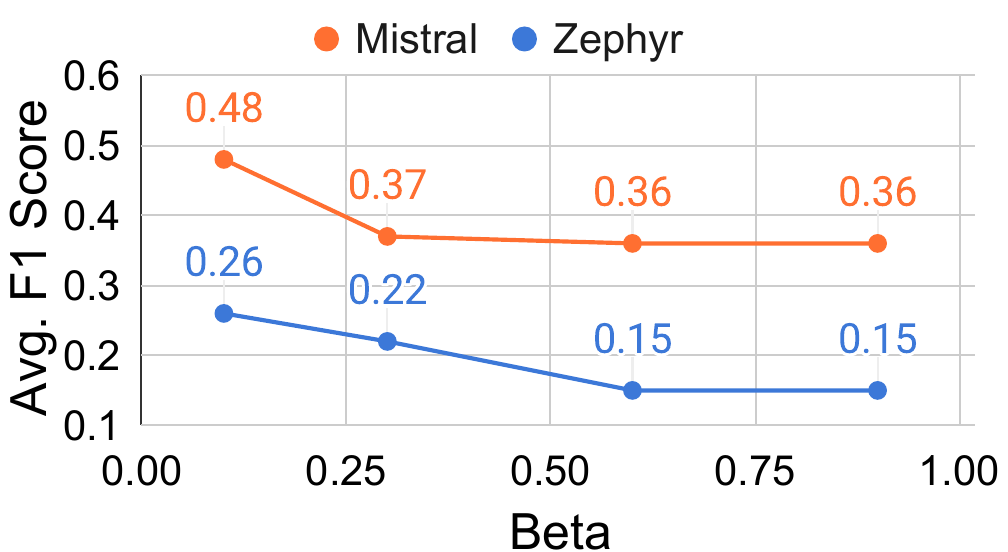}
    \end{subfigure}
    \caption{DPO and IPO performance as a function of beta. This figure depicts how the beta hyper-parameter affects the average f1-socre across three classification fields of DPO and IPO aligned models. We found that both DPO and IPO performances were influenced by beta adjustments. Specifically, a beta of 0.1 optimized results for DPO, while a higher beta of 0.9 notably reduced the f1-score. Similarly, IPO performed best with a beta of 0.1, and increasing the beta decreased the f1-score.}
    \label{fig:app_exp2}
\end{figure}

To complement the experiments in Section \ref{exp2}, we measured the average f1-score across the three classification fields to analyze the effect of the beta hyper-parameter on DPO and IPO. We found that the performance of DPO and IPO is sensitive to the choice of beta. As depicted in Figure \ref{fig:app_exp2}, for DPO, we observed that a beta of 0.1 yielded the best results: Mistral achieved an f1-score of 0.56, and Zephyr achieved an average f1-score of 0.56. Conversely, a larger beta value, such as 0.9, diminished the performance of the models. Zephyr suffered a large loss of 0.13 in average f1-score from using 0.9 instead of 0.3. As opposed to IPO, we observed that a beta of 0.1 produced the best performance (Figure \ref{fig:app_exp2}). A larger choice of beta in IPO almost always came with a loss of performance. As beta increases, Mistral's f1-score dropped from 0.48 to 0.36, while Zephyr's f1-score dropped from 0.26 to 0.15.
